# Supplementary material for: Characterizing the deep uncertainties surrounding coastal flood hazard projections: A case study for Norfolk, VA
Source: arXiv:1812.04673 ancillary file (2019-06-10)
Supplement: Supplementary file 1 [file Supplementary-mat.pdf]

# Supporting Information for: Characterizing the deep uncertainties surrounding coastal flood hazard projections: A case study for Norfolk, VA

Kelsey L. Ruckert<sup>1</sup>, Vivek Srikrishnan<sup>1</sup>, and Klaus Keller<sup>1,2,\*</sup>

<sup>1</sup>Earth and Environmental Systems Institute, The Pennsylvania State University,  
University Park, PA, 16802, USA

<sup>2</sup>Department of Geosciences, The Pennsylvania State University, University Park, PA,  
16802, USA

\*Corresponding author: klaus@psu.edu

## Contents of this file

1. Table S1
2. Figure S1
3. Figure S2

## Introduction

This supporting information provides a table of the variables used to create a range of plausible sea-level rise scenarios, a figure depicting a simple diagnostic test that evaluates the reliability of our projections out to 2200, and a figure depicting historical observations from the Sewell's Point tide gauge.

Table S1: Comparison of key variables and information used to create a range of plausible scenarios with the National Research Council (1987) global mean sea-level rise model for USACE (2011, 2013, 2014), Parris et al. (2012), Hall et al. (2016), and Sweet et al. (2017).

| <b>Study:</b>                   | <b>USACE [2011;<br/>2013; 2014]</b> | <b>Parris et<br/>al. [2012]</b> | <b>Hall et<br/>al. [2016]</b> | <b>Sweet et<br/>al. [2017]</b> |
|---------------------------------|-------------------------------------|---------------------------------|-------------------------------|--------------------------------|
| Reference year                  | 2000                                | 2000                            | 2000                          | 2000                           |
| Eustatic SLC rate (mm/yr)       | 1.7                                 | 1.7                             | 1.7                           | 3                              |
| Local relative SLC rate (mm/yr) | 4.44                                | 4.44                            | 4.44                          |                                |
| Rate of VLM                     | 2.61                                | 2.61                            | 2.61                          | 2.47                           |
| Constant b (m/yr <sup>2</sup> ) | 2.71 <sup>-5</sup>                  | 2.71 <sup>-5</sup>              | 2.71 <sup>-5</sup>            | 2.00 <sup>-5</sup>             |
|                                 | 1.13 <sup>-4</sup>                  | 8.71 <sup>-5</sup>              | 7.00 <sup>-5</sup>            | 7.00 <sup>-5</sup>             |
|                                 |                                     | 1.56 <sup>-4</sup>              | 1.13 <sup>-4</sup>            | 1.20 <sup>-4</sup>             |
|                                 |                                     |                                 | 1.56 <sup>-4</sup>            | 1.70 <sup>-4</sup>             |
|                                 |                                     |                                 |                               | 2.20 <sup>-4</sup>             |
| Eustatic SLC in 2100 (m)        | 0.17 - 1.48                         | 0.17 - 1.98                     | 0.17 - 1.98                   | 0.3 - 2.5                      |
| Local relative SLC in 2100 (m)  | 0.44 - 1.76                         | 0.44 - 2.25                     | 0.44 - 2.25                   | 0.61 - 3.53                    |

*Note.* SLC: sea-level change; VLM: vertical land movement

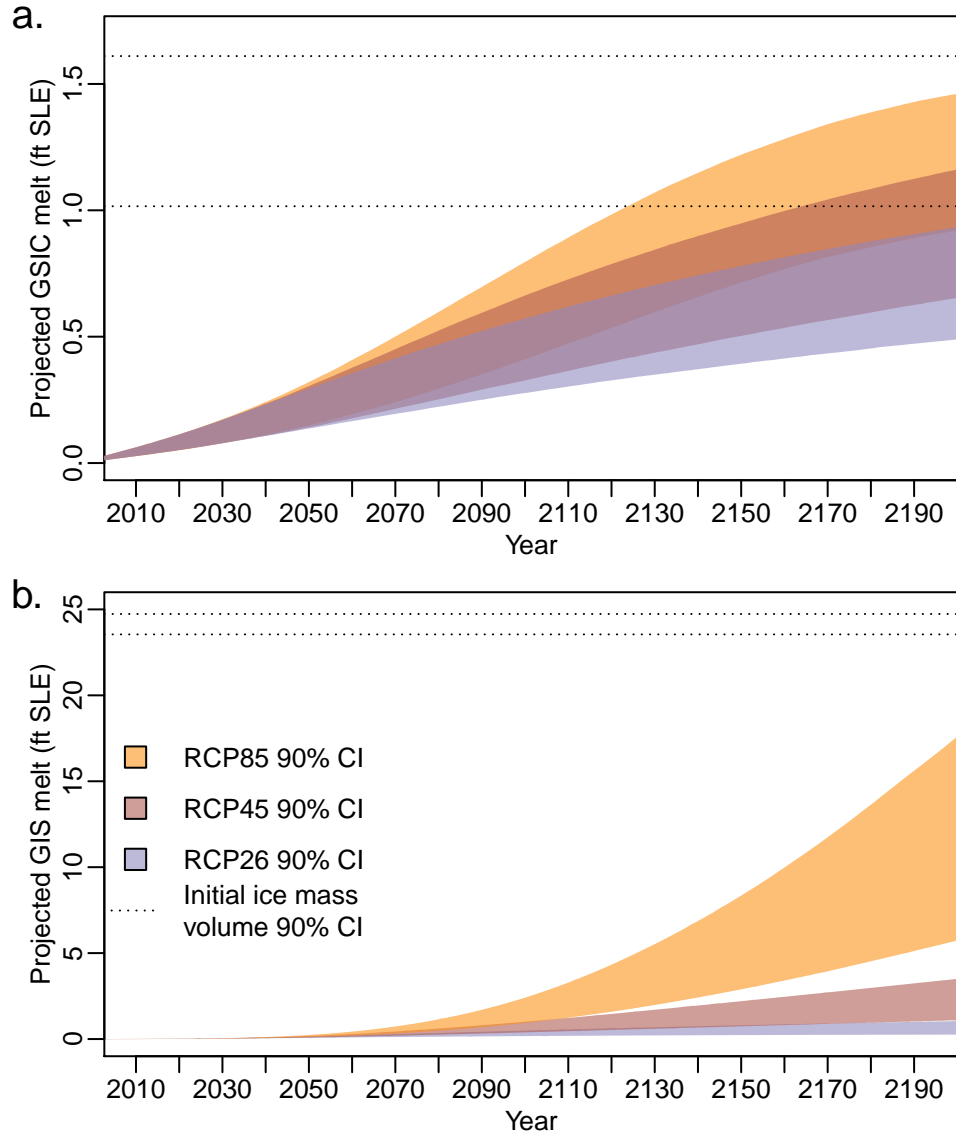

Figure S1: 90% credible intervals of ice mass projections (glaciers and small ice caps in panel a and Greenland ice sheet in panel b) in sea-level equivalence in comparison to the 90% credible interval of initial ice mass from *Wong et al.* [2017].

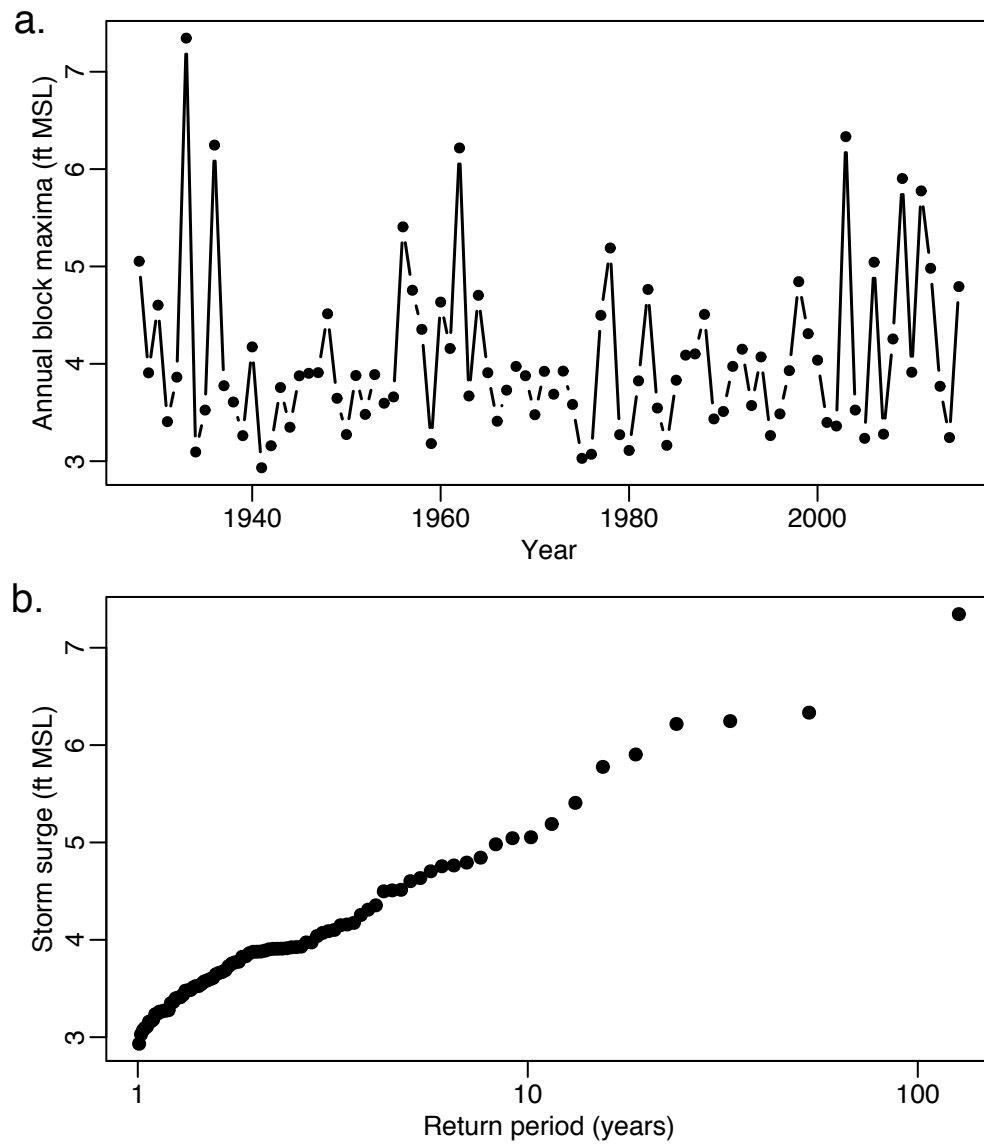

Figure S2: Maximum recorded sea-level anomaly in a year, the annual block maxima, for the Sewell's Point tide gauge (panel a) and the associated return periods for these storm surges (panel b).
